# Supplementary material for: A recursively partitioned approach to architecture-aware ZX Polynomial synthesis and optimization
Source: arXiv:2303.17366 source file (2023-03-31)
Supplement: Supplementary file 1 [file cx_commutation_rules.tex]

We conducted an automated proof following \cite{PauliOpt}. At the base of it is the fact that any Pauli gadget is defined as in Figure~\ref{fig:pauli_gadget_zx}. Hence we can express any Pauli gadget by the matrix exponentiation: $\exp (-i\frac{\theta}{2}G_P)$, where $G_P = \bigotimes_{i = 0}^n P_i$ and $P \in \{X, Y, Z, I\}^n$.
We denote a CNOT with control c and target t as $CX_{c, t}$, a CY as $CY_{c, t}$, and a CZ as $CZ_{c, t}$. In the following, we will outline the process for our proof for $CX_{c, t}$. Nevertheless, the procedure is equivalent to $CY_{c, t}$ and $CZ_{c, t}$, which will nevertheless be omitted for conciseness.
\begin{equation}\label{eq:paul_cx_commutation}
	CX_{c, t} G_p =  G'_p CX_{c, t}
\end{equation}
Hence given Eq.~\eqref{eq:paul_cx_commutation}, we can get to the following conclusion:
\begin{align*}
	CX_{c, t}P(G_P) & = CX_{c, t}\exp (-i \frac{\theta}{2} G_P) \\
			& = \exp (-i \frac{\theta}{2} CX_{c, t} G_P) \\
			& = \exp (-i \frac{\theta}{2} G'_P CX_{c, t}) \\
			& = \exp (-i \frac{\theta}{2}G'_P) CX_{c, t}
\end{align*}
So all we need to find is the set of Paulis that provides $G'_p$. Then, by the topological independence in ZX-calculus, we can argue that the control and target are always neighboring.
Next, it is sufficient just to consider the qubits of the control and target, since $CX_{c, t} = I \otimes CX \otimes I$, hence:
\begin{align*}
	& CX_{c, t} G_p \\
	& = (I \otimes CX \otimes I)(\bigotimes_{i = 0}^n P_i)\\
	& = (I \otimes CX \otimes I)((\bigotimes_{i = 0}^c P_i) \otimes (P_c \otimes P_t) \otimes (\bigotimes_{i = t+1}^n P_i)) \\
	& = (I \cdot (\bigotimes_{i = 0}^c P_i)) \otimes (CX (P_c \otimes P_t)) \otimes (I \cdot (\bigotimes_{i = t+1}^n P_i))\\
	& = ((\bigotimes_{i = 0}^c P_i) \cdot I) \otimes ((P'_c \otimes P'_t) CX) \otimes ((\bigotimes_{i = t+1}^n P_i) \cdot I)\\
	& = ((\bigotimes_{i = 0}^c P_i) \otimes (P'_c \otimes P'_t) \otimes (\bigotimes_{i = t+1}^n P_i)) \cdot (I \otimes CX \otimes I) \\
	& =  G'_p CX_{c, t}
\end{align*}
So we can conclude that propagating a controlled gate trough a Pauli gadget will affect the control and target qubits. With that in mind, one can see that it is sufficient to evaluate Eq.~\eqref{eq:proof_equation} and find the corresponding tuples $(P_0, P_1)$ and $(P'_0, P'_1)$ for Pauli gadgets.
\begin{equation}\label{eq:proof_equation}
	CX \exp(-i\frac{\theta}{2}(P_0 \otimes P_1)) \overset{!}{=} \exp(-i\frac{\theta}{2}(P'_0 \otimes P'_1)) CX
\end{equation}
We used sympy to verify the unitaries up to the argument $-i\frac{\theta}{2}$. An example output of such a proof can be found in Figure~\ref{fig:example_pauli_gadget}. The commutation rules we derived with this method can be found in Figure~\ref{fig:cx_commutation_rules}~\ref{fig:cy_commutation_rules}~\ref{fig:cz_commutation_rules}
\begin{figure}
	\centering
	\includegraphics[width=0.9\linewidth]{pgs_relations/proof_cx/proof_XX_XI.pdf}
	\caption{Example proof for the pauli gadget $\exp(-i\frac{\theta}{2}(X \otimes X))$. With the produced unitaries by sympy.}\label{fig:example_pauli_gadget}
\end{figure}
\begin{figure}[ht]
	\centering
	\includegraphics[width=0.4\linewidth]{pgs_relations/proof_cx/pgs_XX_XI.pdf}
	\includegraphics[width=0.4\linewidth]{pgs_relations/proof_cx/pgs_XY_YZ.pdf}
	\includegraphics[width=0.4\linewidth]{pgs_relations/proof_cx/pgs_XZ_YY.pdf}
	\includegraphics[width=0.4\linewidth]{pgs_relations/proof_cx/pgs_XI_XX.pdf}
	\includegraphics[width=0.4\linewidth]{pgs_relations/proof_cx/pgs_YX_YI.pdf}
	\includegraphics[width=0.4\linewidth]{pgs_relations/proof_cx/pgs_YY_XZ.pdf}
	\includegraphics[width=0.4\linewidth]{pgs_relations/proof_cx/pgs_YZ_XY.pdf}
	\includegraphics[width=0.4\linewidth]{pgs_relations/proof_cx/pgs_YI_YX.pdf}
	\includegraphics[width=0.4\linewidth]{pgs_relations/proof_cx/pgs_ZX_ZX.pdf}
	\includegraphics[width=0.4\linewidth]{pgs_relations/proof_cx/pgs_ZY_IY.pdf}
	\includegraphics[width=0.4\linewidth]{pgs_relations/proof_cx/pgs_ZZ_IZ.pdf}
	\includegraphics[width=0.4\linewidth]{pgs_relations/proof_cx/pgs_ZI_ZI.pdf}
	\caption{Complete CX Proragation Rules for Pauli Gadgets}
	\label{fig:cx_commutation_rules}
\end{figure}
\begin{figure}[ht]
	\centering
	\includegraphics[width=0.4\linewidth]{pgs_relations/proof_cy/pgs_XX_YZ.pdf}
	\includegraphics[width=0.4\linewidth]{pgs_relations/proof_cy/pgs_XY_XI.pdf}
	\includegraphics[width=0.4\linewidth]{pgs_relations/proof_cy/pgs_XZ_YX.pdf}
	\includegraphics[width=0.4\linewidth]{pgs_relations/proof_cy/pgs_XI_XY.pdf}
	\includegraphics[width=0.4\linewidth]{pgs_relations/proof_cy/pgs_YX_XZ.pdf}
	\includegraphics[width=0.4\linewidth]{pgs_relations/proof_cy/pgs_YY_YI.pdf}
	\includegraphics[width=0.4\linewidth]{pgs_relations/proof_cy/pgs_YZ_XX.pdf}
	\includegraphics[width=0.4\linewidth]{pgs_relations/proof_cy/pgs_YI_YY.pdf}
	\includegraphics[width=0.4\linewidth]{pgs_relations/proof_cy/pgs_ZX_IX.pdf}
	\includegraphics[width=0.4\linewidth]{pgs_relations/proof_cy/pgs_ZY_ZY.pdf}
	\includegraphics[width=0.4\linewidth]{pgs_relations/proof_cy/pgs_ZZ_IZ.pdf}
	\includegraphics[width=0.4\linewidth]{pgs_relations/proof_cy/pgs_ZI_ZI.pdf}
	\caption{Complete CY Proragation Rules for Pauli Gadgets}
	\label{fig:cy_commutation_rules}
\end{figure}
\begin{figure}[ht]
	\centering
	\includegraphics[width=0.4\linewidth]{pgs_relations/proof_cz/pgs_XX_YY.pdf}
	\includegraphics[width=0.4\linewidth]{pgs_relations/proof_cz/pgs_XY_YX.pdf}
	\includegraphics[width=0.4\linewidth]{pgs_relations/proof_cz/pgs_XZ_XI.pdf}
	\includegraphics[width=0.4\linewidth]{pgs_relations/proof_cz/pgs_XI_XZ.pdf}
	\includegraphics[width=0.4\linewidth]{pgs_relations/proof_cz/pgs_YX_XY.pdf}
	\includegraphics[width=0.4\linewidth]{pgs_relations/proof_cz/pgs_YY_XX.pdf}
	\includegraphics[width=0.4\linewidth]{pgs_relations/proof_cz/pgs_YZ_YI.pdf}
	\includegraphics[width=0.4\linewidth]{pgs_relations/proof_cz/pgs_YI_YZ.pdf}
	\includegraphics[width=0.4\linewidth]{pgs_relations/proof_cz/pgs_ZX_IX.pdf}
	\includegraphics[width=0.4\linewidth]{pgs_relations/proof_cz/pgs_ZY_IY.pdf}
	\includegraphics[width=0.4\linewidth]{pgs_relations/proof_cz/pgs_ZZ_ZZ.pdf}
	\includegraphics[width=0.4\linewidth]{pgs_relations/proof_cz/pgs_ZI_ZI.pdf}
	\caption{Complete CZ Proragation Rules for Pauli Gadgets}
	\label{fig:cz_commutation_rules}
\end{figure}
