# Supplementary material for: A recursively partitioned approach to architecture-aware ZX Polynomial synthesis and optimization
Source: arXiv:2303.17366 source file (2023-03-31)
Supplement: Supplementary file 2 [file parity_map.tex]

As a simple example, we examine the effect of a single CNOT in circuit notation, seen in Fig.~\ref{fig:circuit_single_cnot} and parity map notation, seen in Fig.~\ref{fig:parity_map_single_cnot}. In the circuit notation, the $\oplus$ operation is defined as the ubiquitous addition modulo $2$.
\begin{figure}[ht]
	\centering
	\begin{equation*}
		\begin{quantikz}
			\lstick{}_{q_0} & \ctrl{1} & \qw_{q_0} \\
			\lstick{}_{q_1} & \targ{}  & \qw_{q_1 \oplus q_0} \\
			\lstick{}_{q_2} & \qw      & \qw_{q_2} \\
		\end{quantikz}
	\end{equation*}
	\caption{One can see, that the application of a CNOT from the right corresponds to the addition of qubit 0 to qubit 1}\label{fig:circuit_single_cnot}
\end{figure}
In parity map notation, we represent the effect of the CNOT by the state of the system before and after its application. 
For convenience, the initial state of a system is the identity.
\begin{figure}[ht!]
\centering
\begin{align*}
\begin{pNiceMatrix}[columns-width=10pt,first-col,nullify-dots]
q_0 & 1   & 0   & 0\\
q_1 & 0   & 1   & 0\\
q_2 & 0   & 0   & 1\\
\end{pNiceMatrix} \longrightarrow 
\begin{pNiceMatrix}[columns-width=10pt,first-col,nullify-dots]
q_0 & 1   & 0   & 0\\
q_1 \oplus q_0 & 1   & 1   & 0\\
q_2 & 0   & 0   & 1\\
\end{pNiceMatrix}
\end{align*}
\caption{State of system before CNOT application (left) and after (right)}\label{fig:parity_map_single_cnot}
\end{figure}
We can then represent the effect of a sequence of CNOTs in this notation. 
We generalize the notation of applying a CNOT operation to the left and right of a parity map in Figs.~\ref{fig:parity_maps_circuits_left} and ~\ref{fig:parity_maps_circuits_right}, where a CNOT applied from the right is row addition and from the left is column addition.
\begin{figure}[ht]
	\centering
	\begin{equation*}\label{eq:parity_maps}
		\begin{quantikz}[row sep=0.5em]
			\lstick{}& \qw 		& \gate[5, nwires=3 ][1cm]{P}		& \qw       & \qw           & \qw\\
			\lstick{}& \qw 		&                            		& \qw{i}    & \ctrl{2}      & \ghost{\targ{}}\\
			\lstick{}& \vdots 	&                            		& \vdots    &               & \\
			\lstick{}& \qw 		&                            		& \qw{j}    & \targ{}       & \ghost{\targ{}}\\
			\lstick{}& \qw 		&                           		& \qw       & \qw           & \qw\\
		\end{quantikz}
		=
		\begin{quantikz}[row sep=0.5em]
			\lstick{}& \qw 		& \gate[5, nwires=3 ][1cm]{P'}		& \qw       & \qw           & \qw\\
			\lstick{}& \qw 		&                            		& \qw{i}    & \qw    & \ghost{\targ{}}\\
			\lstick{}& \vdots 	&                            		& \vdots    &               & \\
			\lstick{}& \qw 		&                            		& \qw{j}    & \qw       & \ghost{\targ{}}\\
			\lstick{}& \qw 		&                           		& \qw       & \qw           & \qw\\
		\end{quantikz}
		\implies
		P \xrightarrow[]{P'_j = P_i \oplus P_j} P'
	\end{equation*}	
	\caption{We can see, the effect of a CNOT (present to the \textit{right} of the parity map) as a \textit{row-addition} from control to target}\label{fig:parity_maps_circuits_left}
\end{figure}
We can incorporate the CNOT from the \textit{right} of this parity map, which will provide the map $P_{i, j}$. Since a column addition can then be expressed as $P_{i, j} \cdot P$, it suffices to perform this column addition on our parity map.
Given the concept discussed in the previous figure and the fact that a column addition can be expressed as $P_{i, j} \cdot P$, where $P_{i, j}$ describes the parity map, after application of one CNOT to the \textit{left} (row addition). We can find the application of a CNOT to the \textit{left}, by Figure \ref{fig:parity_maps_circuits_right}.
\begin{figure}[ht]
	\centering
	\begin{equation*}\label{eq:parity_maps}
		\begin{quantikz}[row sep=0.5em]
			\lstick{}& \qw 		& \qw      & \gate[5, nwires=3 ][1cm]{P}	& \qw           & \qw\\
			\lstick{}& \qw 		& \ctrl{2} &                             	& \qw{i}	& \ghost{\targ{}}\\
			\lstick{}& \vdots 	& \vdots   &                            	&               & \\
			\lstick{}& \qw 		& \targ{}  &                            	& \qw{j}        & \ghost{\targ{}}\\
			\lstick{}& \qw 		& \qw      &                           		& \qw           & \qw\\
		\end{quantikz}
		=
		\begin{quantikz}[row sep=0.5em]
			\lstick{}& \qw 		& \gate[5, nwires=3 ][1cm]{P'}		& \qw                  & \qw\\
			\lstick{}& \qw 		&                            		& \qw{i}        & \ghost{\targ{}}\\
			\lstick{}& \vdots 	&                            		& \vdots                 & \\
			\lstick{}& \qw 		&                            		& \qw{j}           & \ghost{\targ{}}\\
			\lstick{}& \qw 		&                           		& \qw                  & \qw\\
		\end{quantikz}
		\implies
		P \xrightarrow[]{P'_{:, j} = P_{:, i} \oplus P_{:, i}} P' \quad
	\end{equation*}	
	\caption{We can see, the effect of a CNOT (present to the \textit{right} of the parity map) as a \textit{column-addition} from control to target}\label{fig:parity_maps_circuits_right}
\end{figure}
