# Supplementary material for: A recursively partitioned approach to architecture-aware ZX Polynomial synthesis and optimization
Source: arXiv:2303.17366 source file (2023-03-31)
Supplement: Supplementary file 3 [file pauli_polynomials.tex]

Those familiar with optimization algorithms, such as the Quantum Approximate Optimization Algorithm, can easily identify that the $Z$ and $X$ phase gadgets are simply circuit representations of the ubiquitous $e^{-i\alpha Z^{\otimes n}}$ and $e^{-i\alpha X^{\otimes n}}$ rotation operators in matrix exponential representation.
Pauli gadgets describe a natural extention of phase gadgets, allowing an arbitrary Pauli string in the exponential instead of a repeated $Z$ or $X$ Pauli string; the legs of a pauli gadget may not be strictly Z or X spiders. 
Instead, they can be composed of a combination of X, Y or Z legs, as seen in Fig.~\ref{fig:pauli_gadget_zx}.
\begin{figure}[ht!]
    \centering
	\begin{equation*}
        \begin{aligned}\label{eq:phase_merging_x}
            \begin{ZX}[math baseline=t1]
                \zxNone{}       &                				& |[pauliPhase]| {\alpha}\\
                \\
                \zxNone{} \rar  & |[pauliX]|  \ar[ruu, bend right] \rar 	& \zxNone{}\\
                \zxNone[a=t1]{} \rar  & |[pauliY]| \ar[ruuu, bend right] \rar 	& \zxNone{}\\
                \zxNone{} \rar 	& |[pauliZ]| \ar[ruuuu, bend right] \rar	& \zxNone{}\\
                \zxNone{} \rar 	& \zxNone{} \rar				& \zxNone{}\\
            \end{ZX}
            = &
            \begin{ZX}[math baseline=t1]
                        &		  &		    & \zxNone{}       & \zxNone{}       	                & \zxZ{\alpha} 			&	    &	\\
                        &		  &		    & \zxNone{}       & \zxNone{}       	                & \zxX{} \ar[u, bend right]	&	    &	\\
                \zxNone{}\rar   & \zxH{}\rar   	  & \zxNone{}\rar   & \zxNone{}\rar   & \zxZ{}  \ar[ru, bend right] \rar 	& \zxNone{}\rar	   		& \zxH{}\rar & \zxNone{}\\
                \zxNone[a=t1]{}\rar   & |[redPlus]| {\oplus} \rar     & \zxNone{}\rar   & \zxNone{} \rar  & \zxZ{} \ar[ruu, bend right] \rar 	& \zxNone{}\rar   		&  |[redPlus]| {\ominus} \rar & \zxNone{}\\
                \zxNone{}\rar   & \zxNone{}\rar   & \zxNone{}\rar   & \zxNone{} \rar  & \zxZ{} \ar[ruuu, bend right] \rar	& \zxNone{}\rar   		& \zxNone{}\rar & \zxNone{}\\
                \zxNone{}\rar   & \zxNone{}\rar   & \zxNone{}\rar   & \zxNone{} \rar  & \zxNone{} \rar				& \zxNone{}\rar   		& \zxNone{}\rar & \zxNone{}\\
            \end{ZX}
        \end{aligned}
    \end{equation*}
    \caption{Pauli gadget representation of $e^{-i\alpha XYZI}$ per notation in  \cite{Cowtan2020} (left) and in ZX-calculus (right)}
    \label{fig:pauli_gadget_zx}
\end{figure}
As similar nomenclature to phase gadgets, we refer to a series of concatenated pauli gadgets as a \textit{Pauli-polynomial}. 
Every Hermitian matrix can be described as the sum of tensor products of weighted Pauli matrices and many quantum algorithms rely on trotterization of such matrices.
This hencefore provides a clear indication, that Pauli-Polynomials can be useful for optimizing variational ansatzes. 
The work of Cowtan et. al \cite{Cowtan2020}, shows an example of quantum chemistry ansatzes being optimized.
At last it is worth to mention, that Cowtan et. al~\cite{Cowtan2020}, has provided a set of rewrite rules in the sense, that one cannot describe the propagation of a CNOT through the Pauli-Polynomial. Nevertheless, as mentioned by him this set is not complete in the sense that it fully describes a propagation of a CNOT through Pauli-Polynomial. We conducted an automated proof based on the formulation by \cite{PauliOpt} to derrive the CX propagation rules through the Pauli-Polynomial. Our approach can be extended towards CY and CZ gates. For a detailed description and proof, see appendix~\ref{sec:pauli_commutation}
