# Supplementary material for: A recursively partitioned approach to architecture-aware ZX Polynomial synthesis and optimization
Source: arXiv:2303.17366 source file (2023-03-31)
Supplement: Supplementary file 4 [file zx_calculus.tex]

\label{app:zx}
The ZX-calculus consists of two "flavors" of tensors (referred to as Z and X spiders), represented in a Penrose graphical notation almost identical to that used to graphically represent tensor networks. 
Z and X spiders (ordered respectively) are defined in Eq.~\eqref{eq:z_x_spiders}.

\begin{equation}\label{eq:z_x_spiders}
\begin{aligned}
	\begin{ZX}
		\leftManyDots{m} \zxZ{\alpha} \rightManyDots{n}
	\end{ZX} &= \ket{0}^{\otimes m}\bra{0}^{\otimes n} + e^{i\alpha}\ket{1}^{\otimes m}\bra{1}^{\otimes n},
	\\
	\begin{ZX}
		\leftManyDots{m} \zxX{\beta} \rightManyDots{n}
	\end{ZX} &= \ket{+}^{\otimes m}\bra{+}^{\otimes n} + e^{i\beta}\ket{-}^{\otimes m}\bra{-}^{\otimes n},
\end{aligned}
\end{equation}

where $\alpha$ and $\beta$ are arbitrary phases $[0, 2\pi)$ and $m$ and $n$ are non-negative integers indicating the number of input and output tensor dimensions.
If the phase of a spider is $0$ or $2\pi$, it is a general convention to denote the  spiders as empty, as shown in Eq.~\eqref{eq:z_x_spiders_empty}.
\begin{equation}\label{eq:z_x_spiders_empty}
\begin{aligned}
	\begin{ZX}
		\leftManyDots{m} \zxZ{} \rightManyDots{n}
	\end{ZX} &= \ket{0}^{\otimes m}\bra{0}^{\otimes n} + \ket{1}^{\otimes m}\bra{1}^{\otimes n}
\\
	\begin{ZX}
		\leftManyDots{m} \zxX{} \rightManyDots{n}
	\end{ZX} &= \ket{+}^{\otimes m}\bra{+}^{\otimes n} + \ket{-}^{\otimes m}\bra{-}^{\otimes n}
\end{aligned}
\end{equation}

As in Penrose notation, two spiders with a connecting leg represent a contraction operation. Unlike in a general tensor network, each leg in ZX-calculus always represents a dimension of 2 and multiple legs connecting the same two tensors are not merged as a simplification step. 
The final component of the ZX-calculus is the Hadamard quantum logic gate, which is represented by a single yellow square.
\begin{equation}
	\begin{ZX}
		\zxNone{}\rar & \zxNone{} \ar[r,H]& \zxNone{}\rar &	\\
	\end{ZX}
\end{equation}
